# Supplementary material for: Effective Representations of Clinical Notes
Source: arXiv:1705.07025 source file (2018-08-16)
Supplement: Supplementary file 1 [file appendix.tex]

\section{Full Results}
\label{app:fullresults}
\scriptsize
\noindent % [inline block 0: 18 envs, 60750 chars -> data_tex | \begin{tabular}{rlll} \toprule...]
\\
