# Supplementary material for: Effective Representations of Clinical Notes
Source: arXiv:1705.07025 source file (2018-08-16)

# Cardiac dysrhythmias

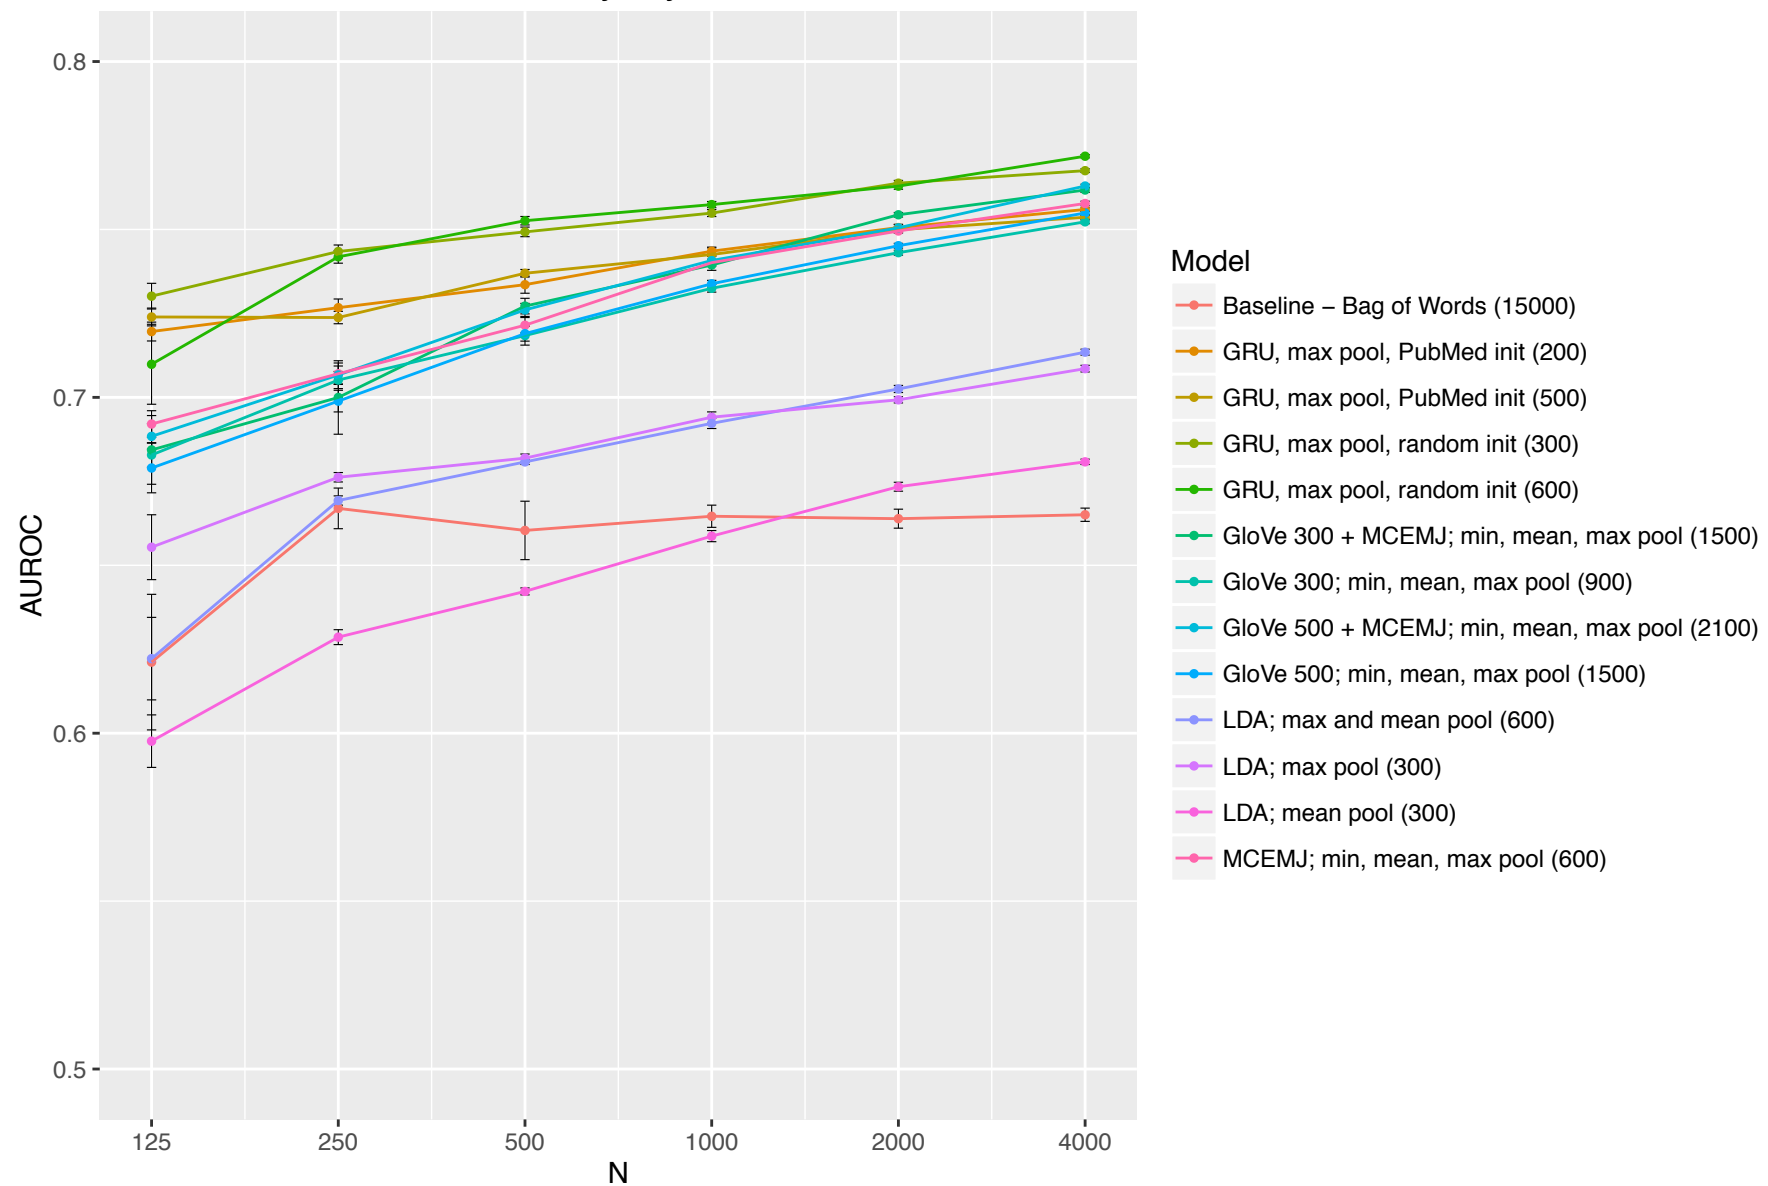

Diabetes mellitus without complication

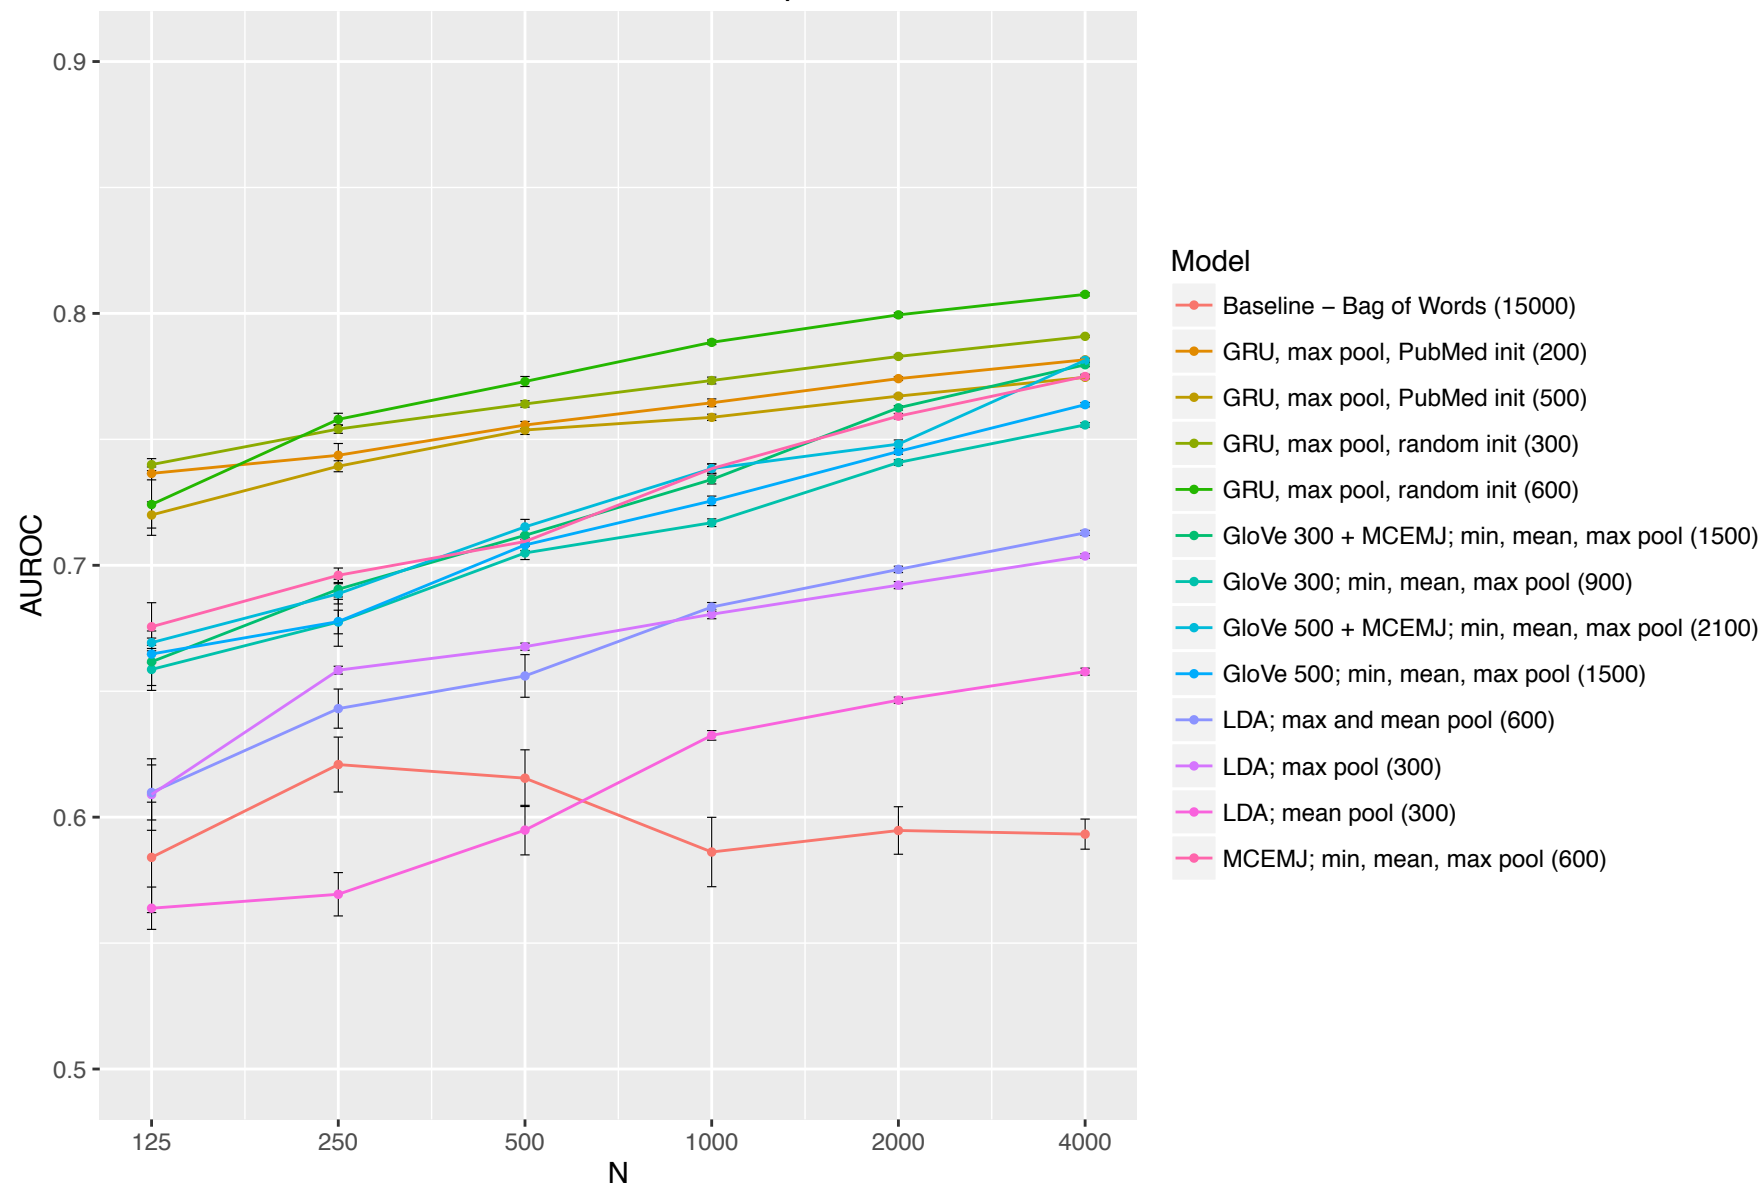

# Disorders of lipid metabolism

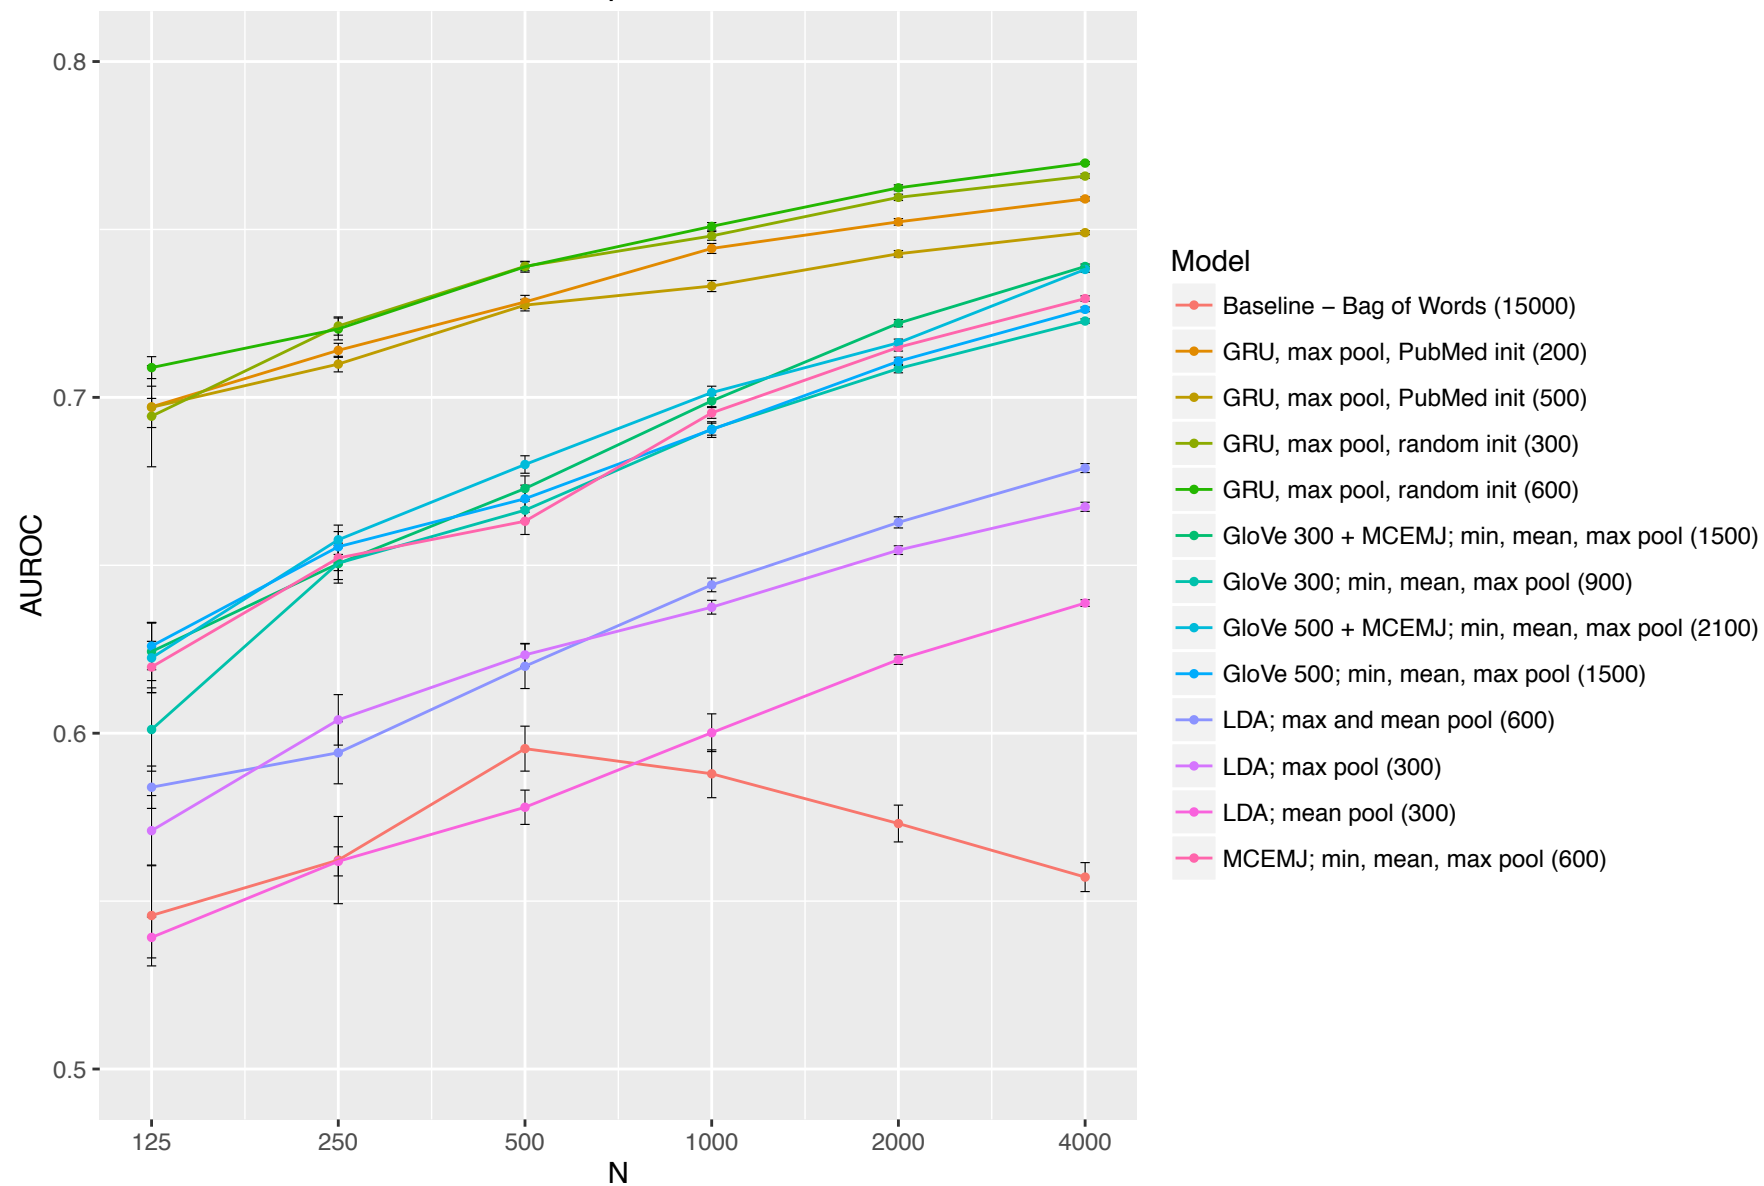

ER visit

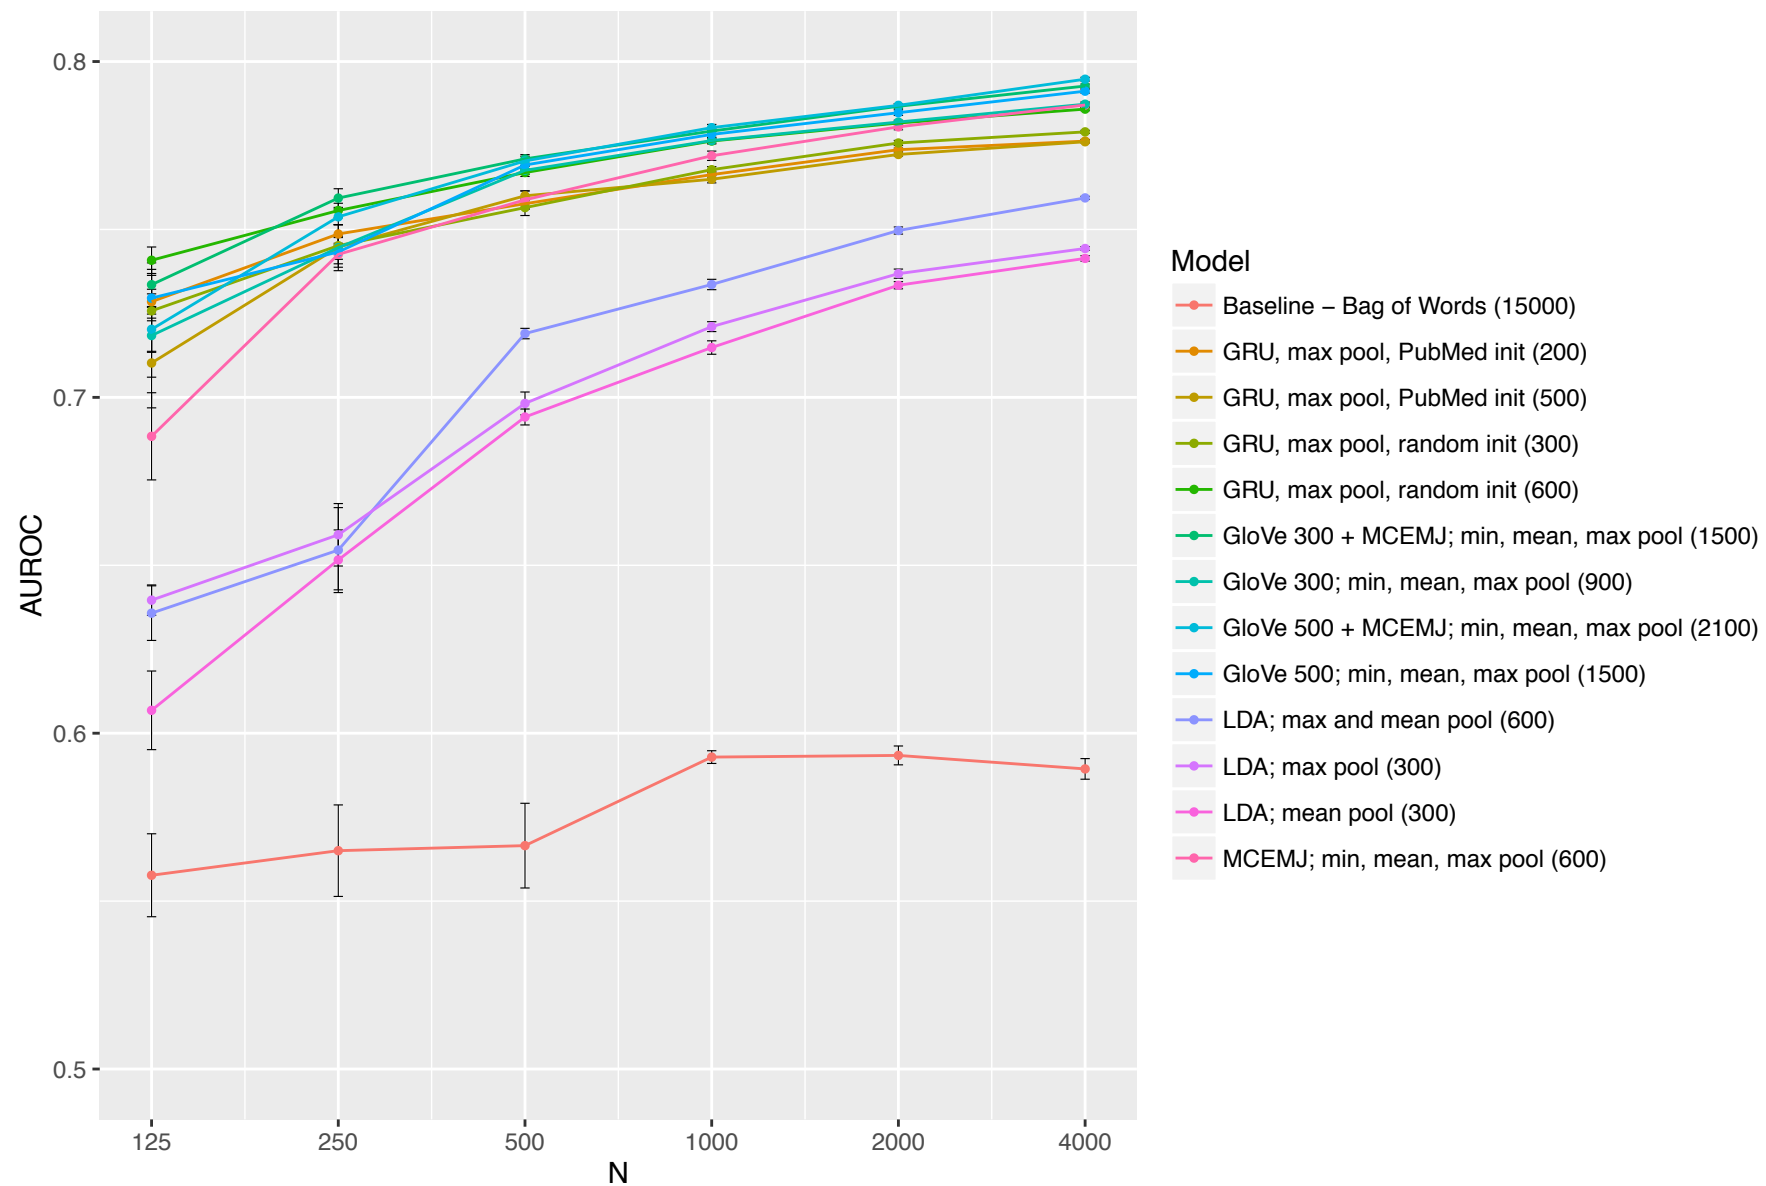

# Essential hypertension

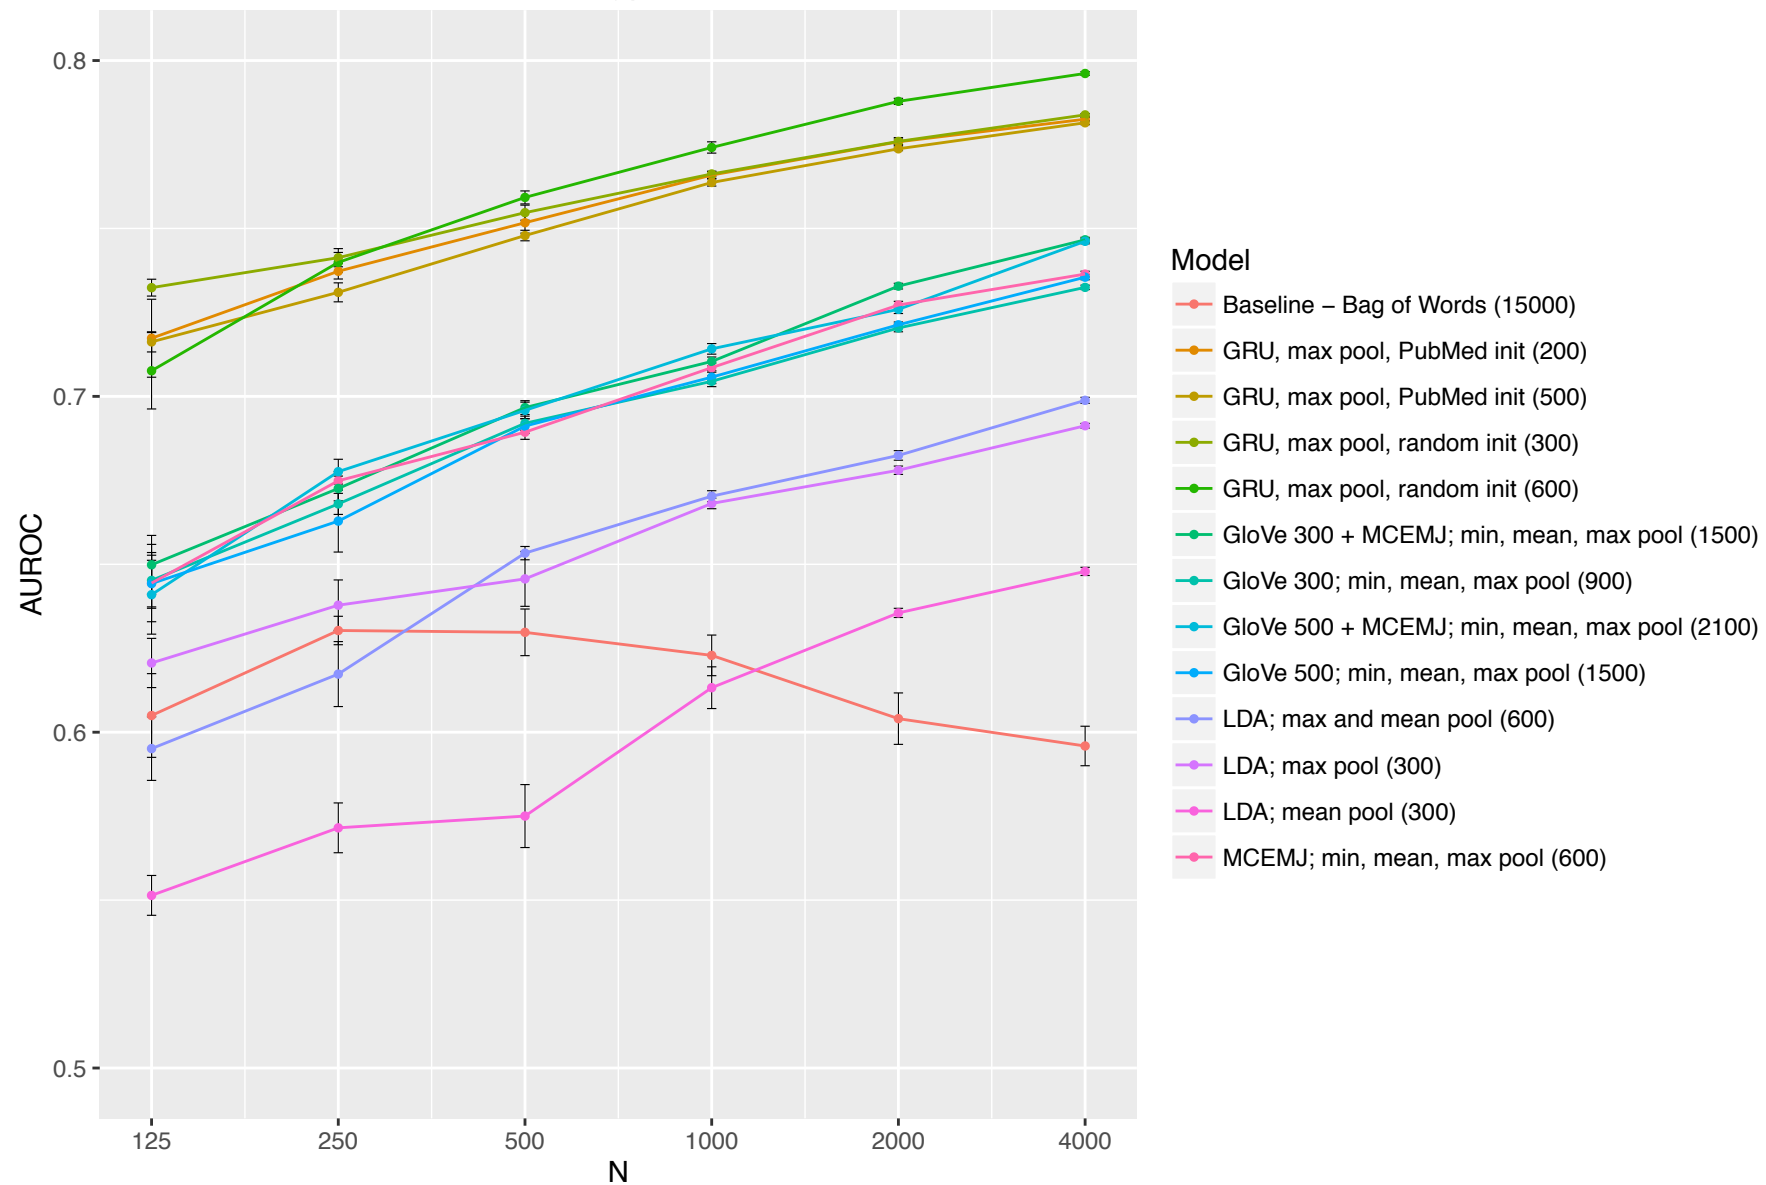

# Inpatient Admission

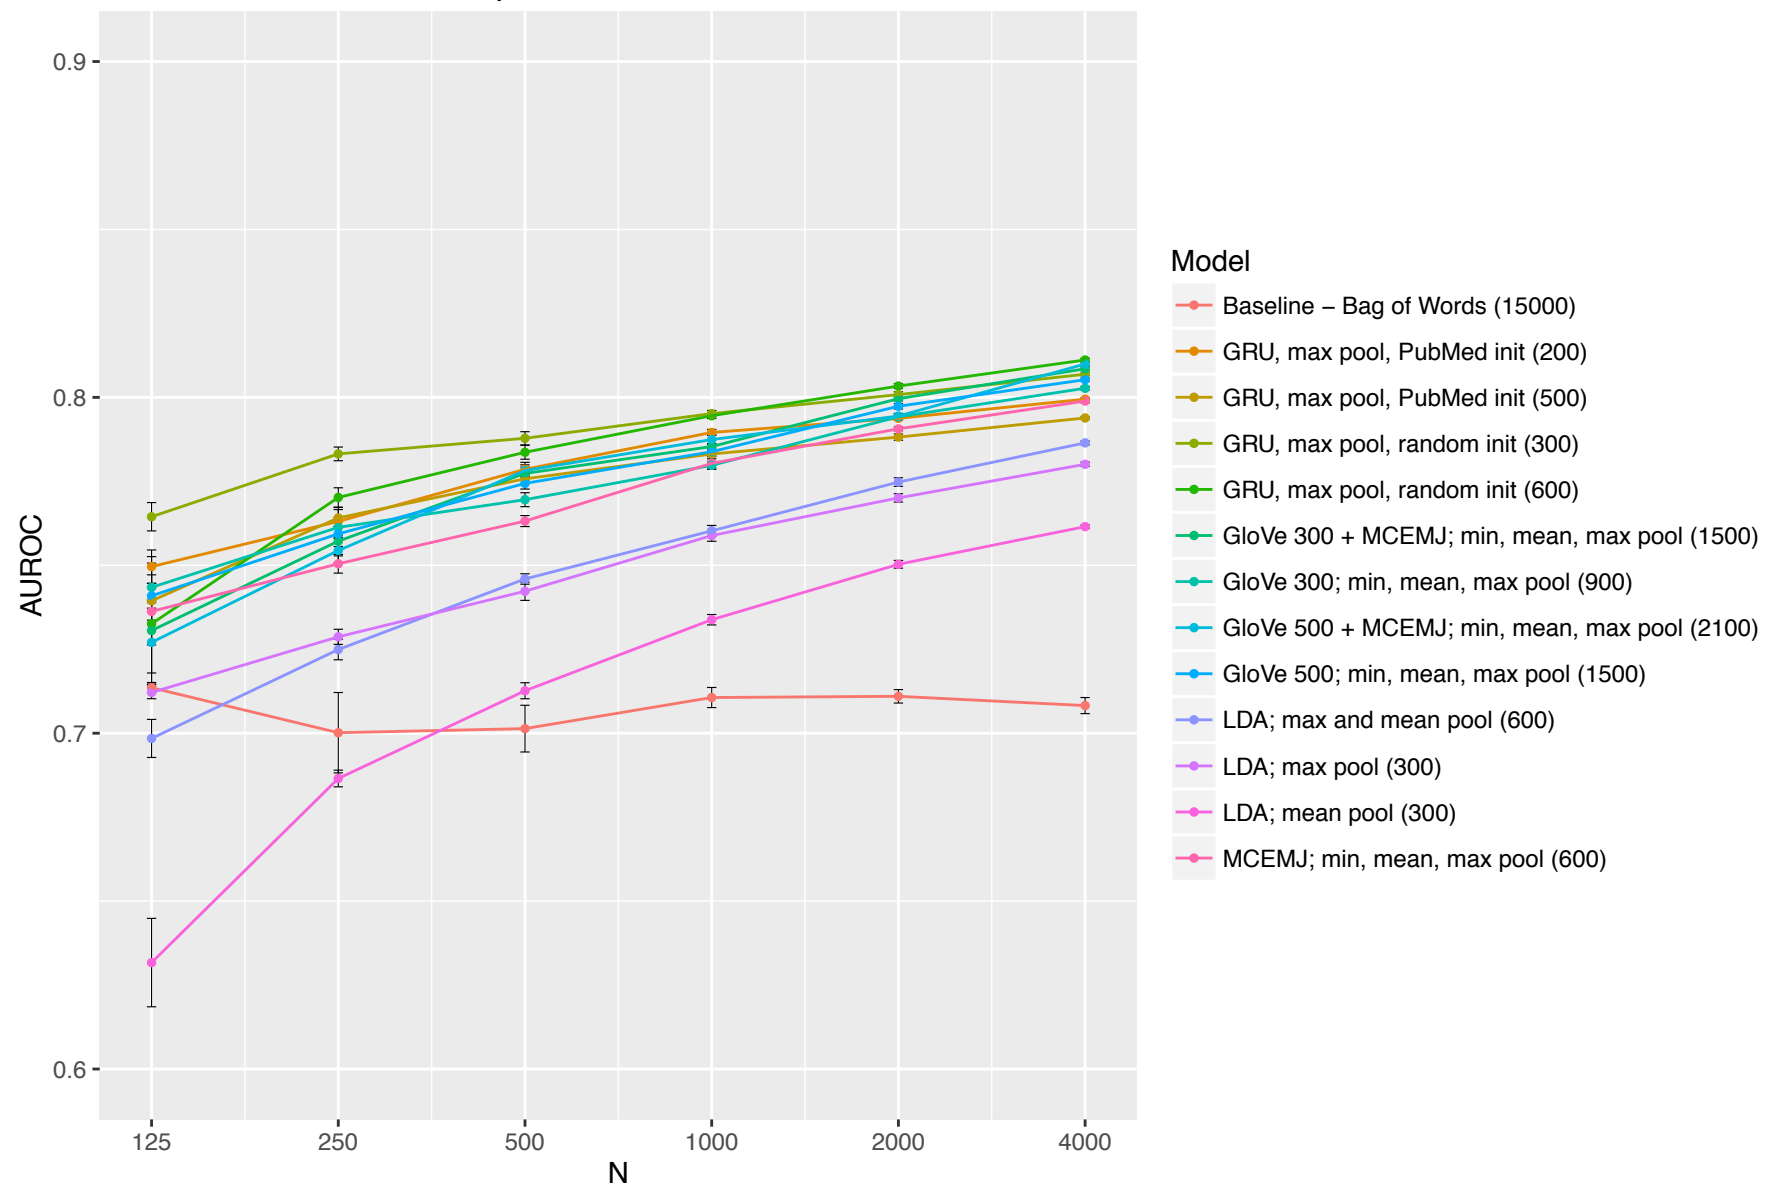

Mortality

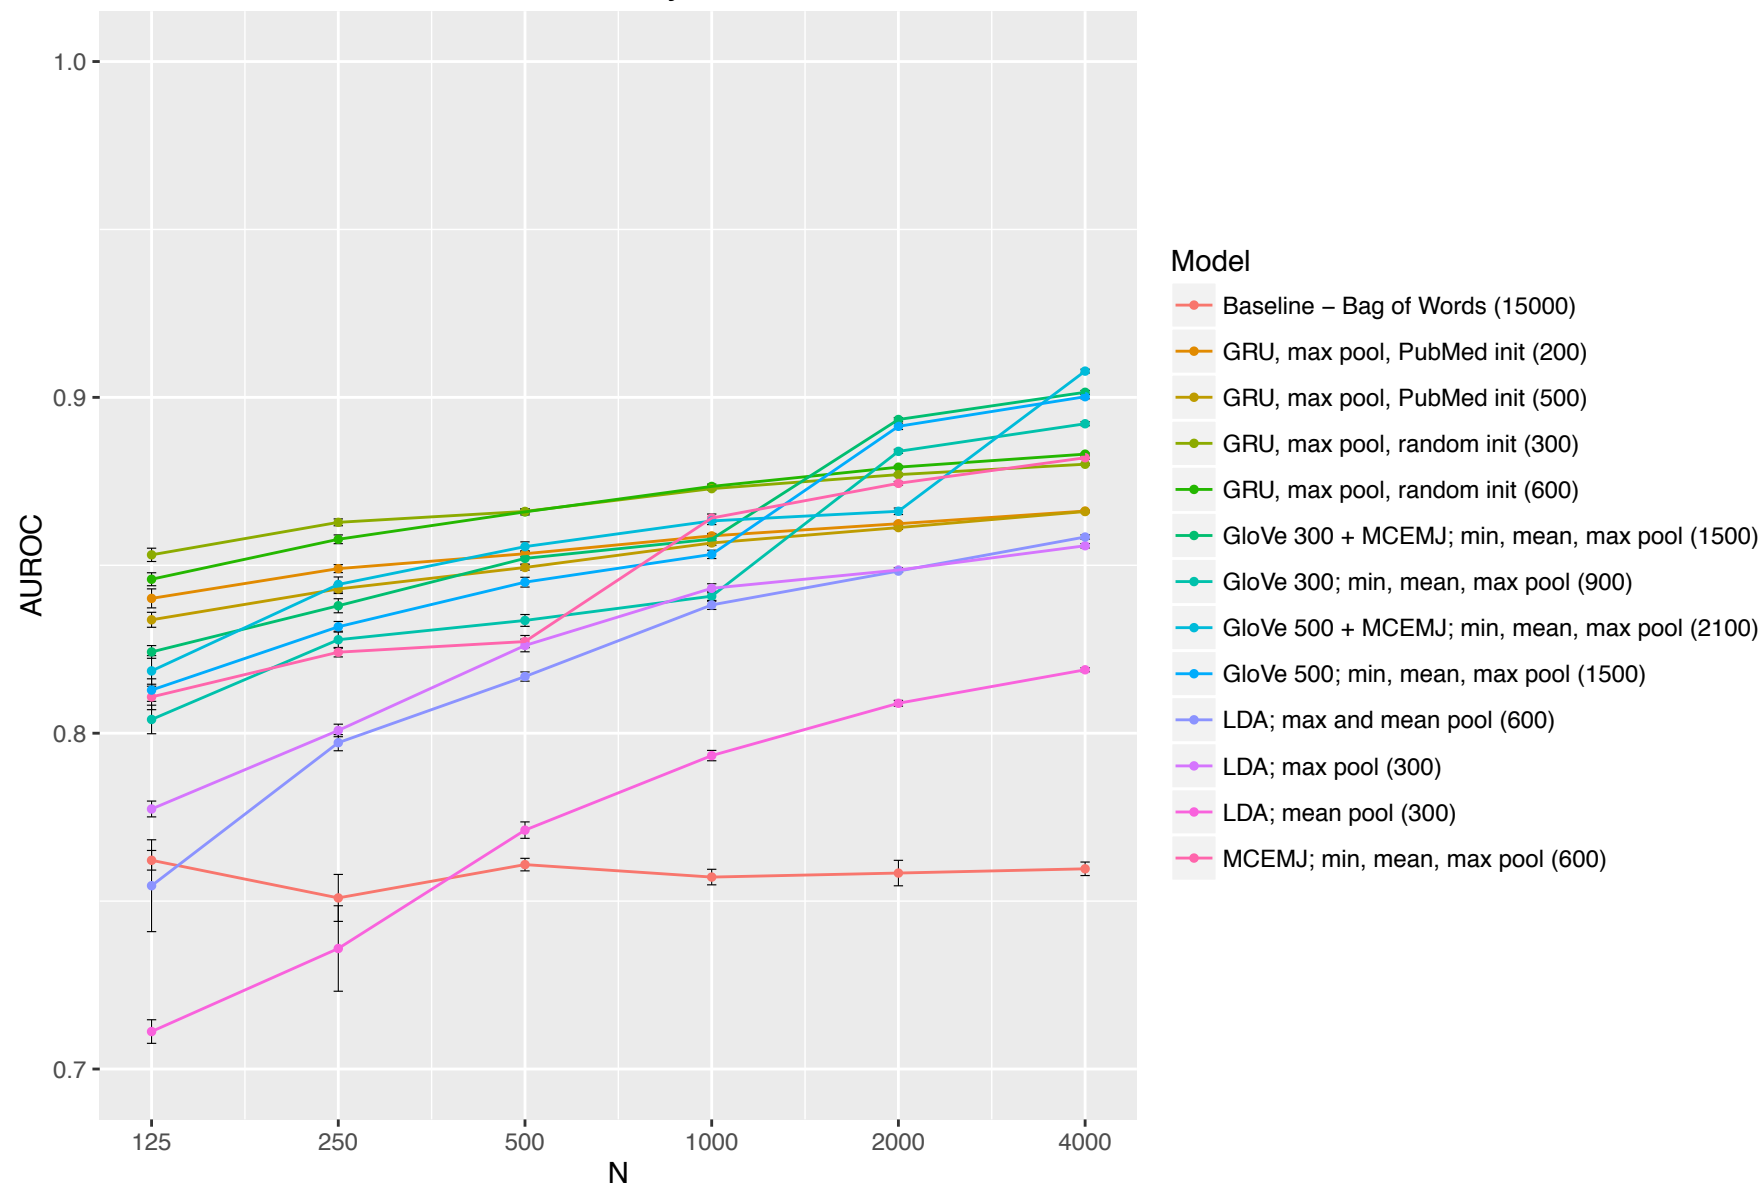

# Spondylosis; intervertebral disc disorders; other back problems

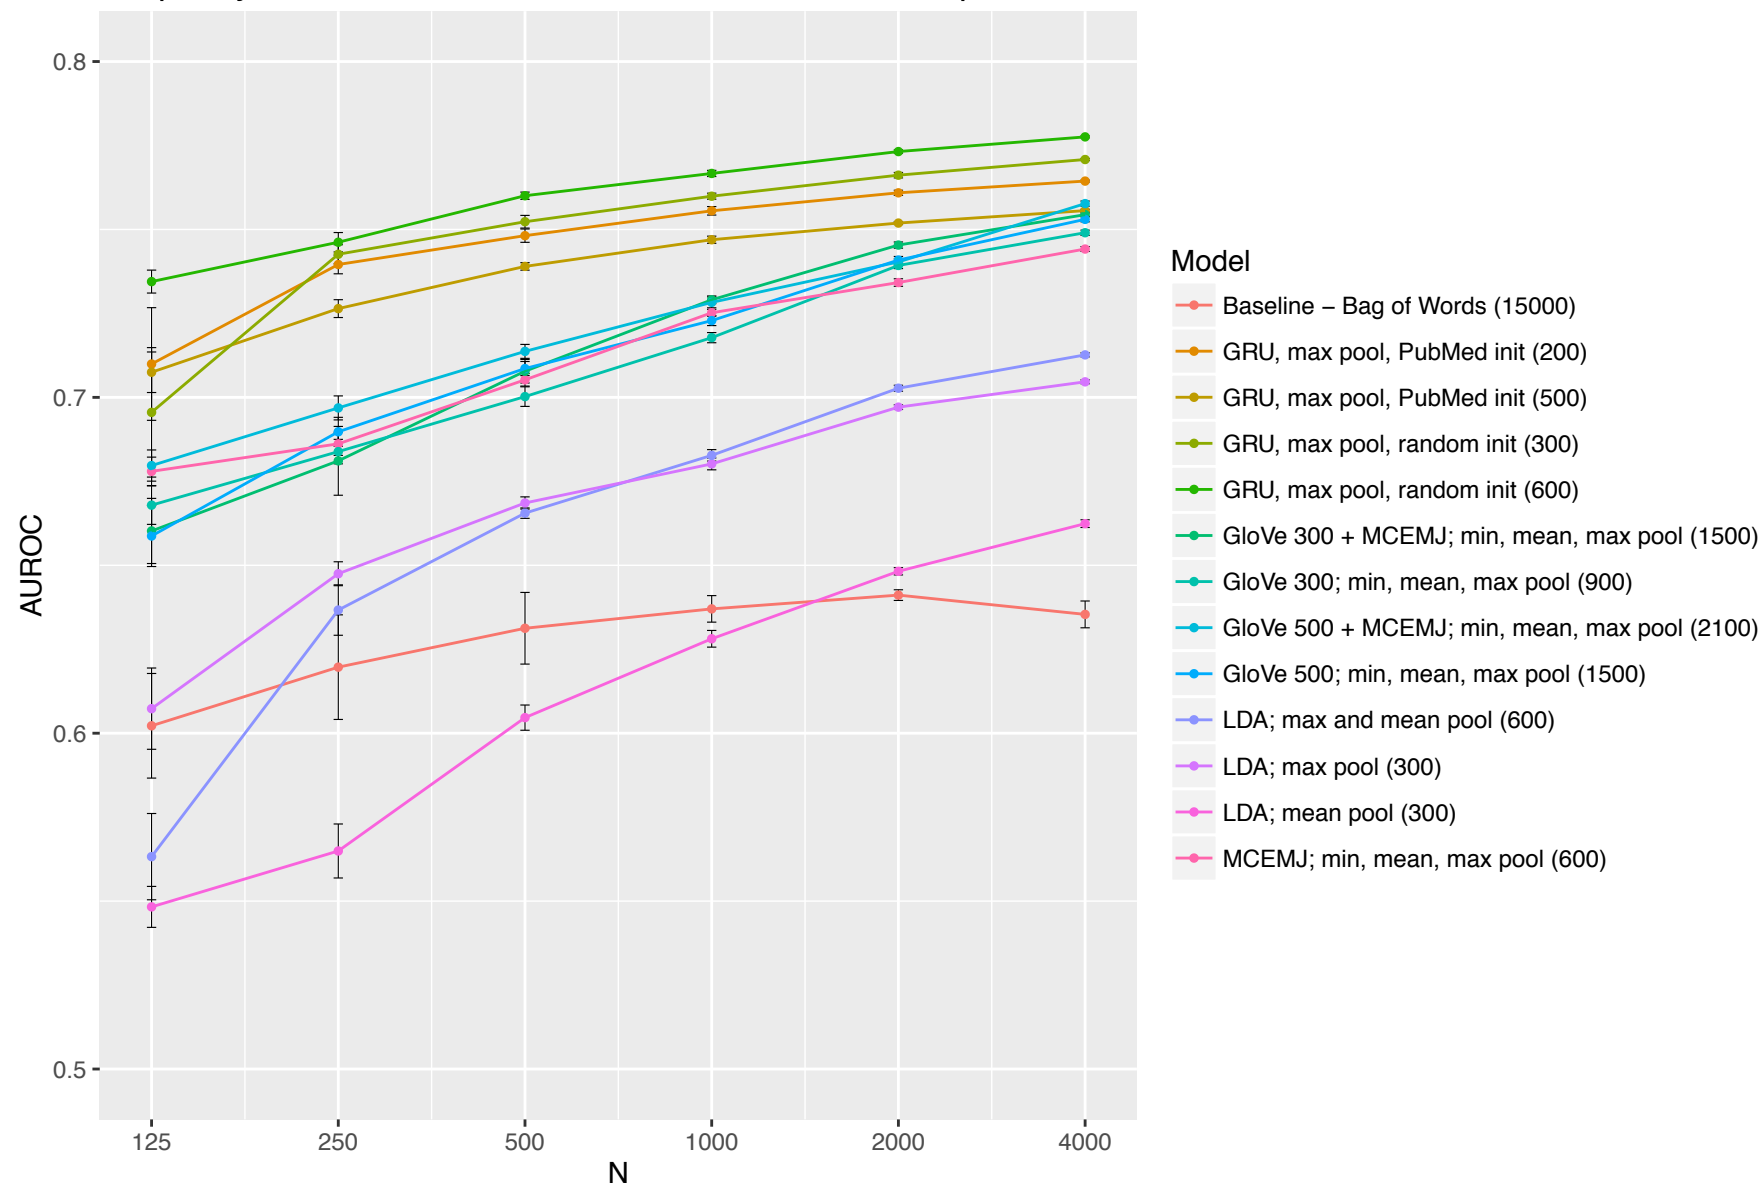

Thyroid disorders

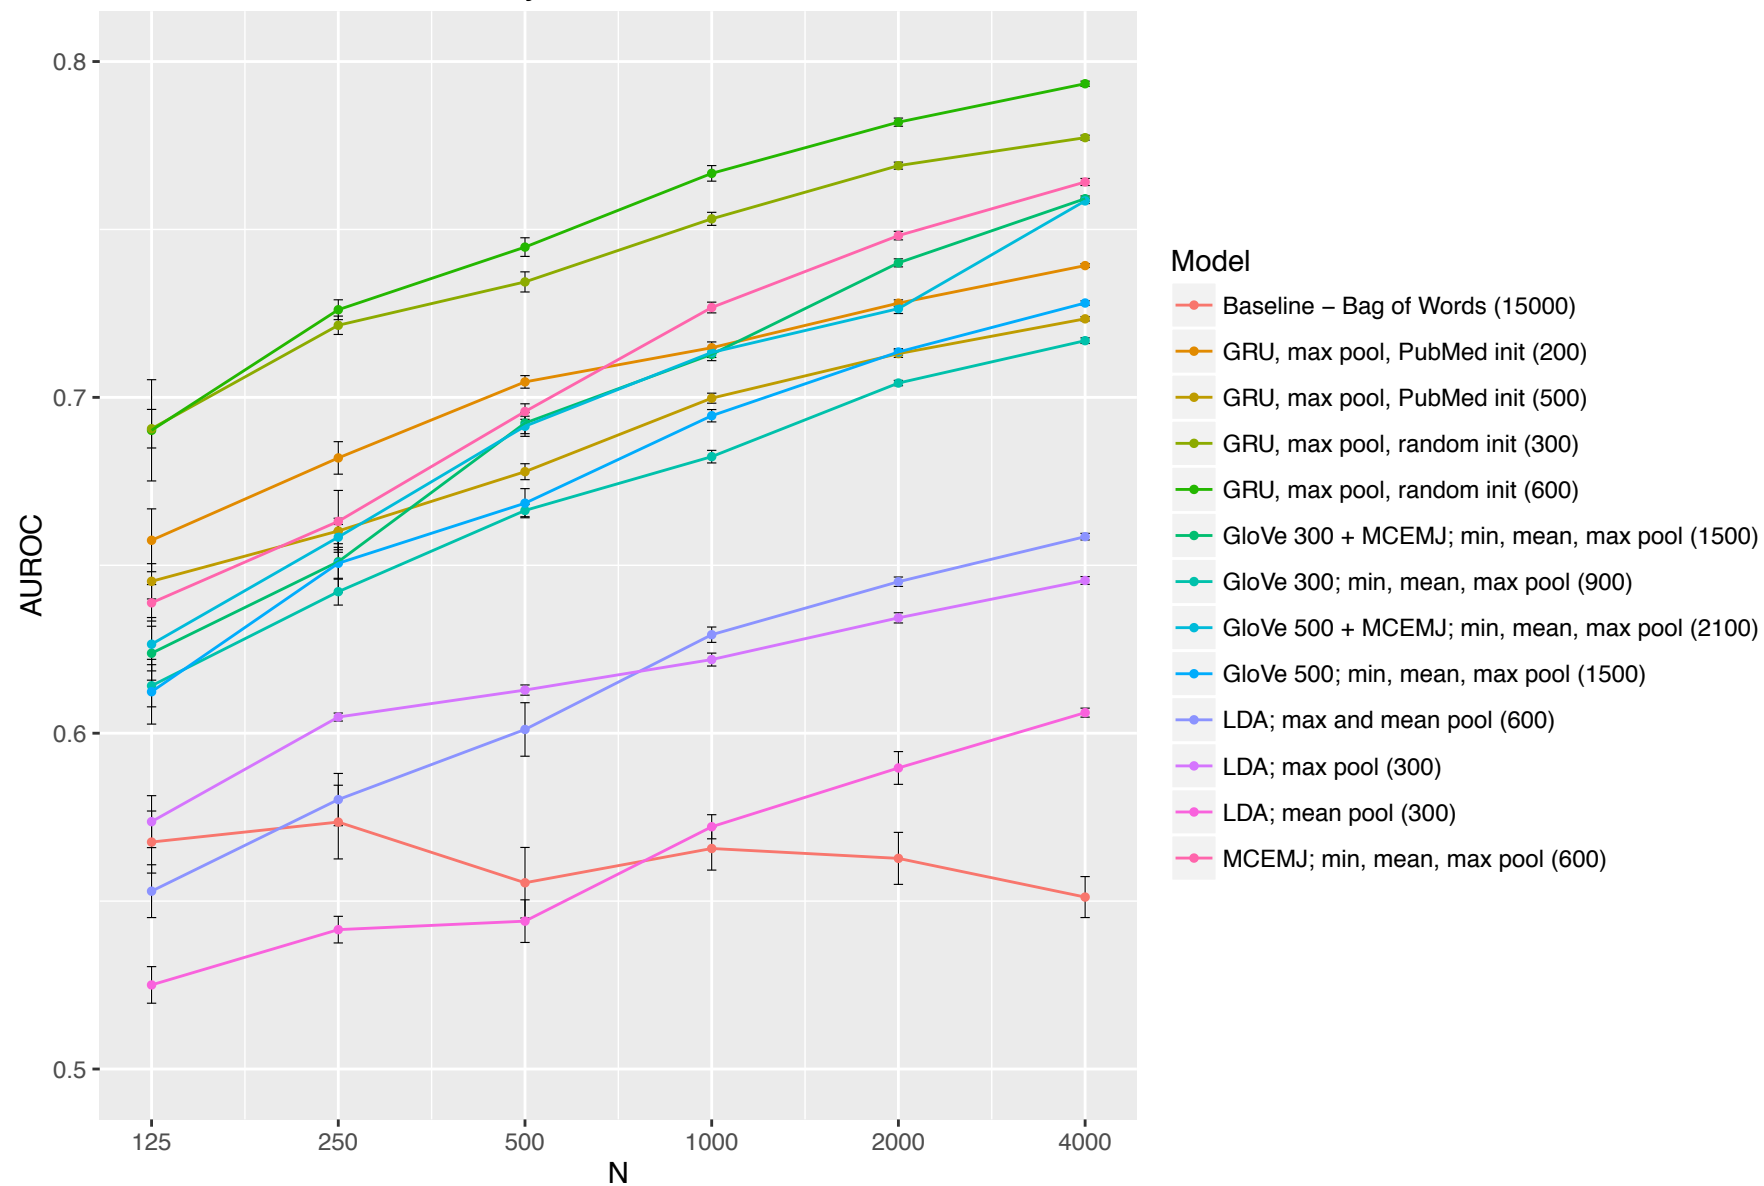

Supplement: Supplementary file 2 [file supplemental-plots-all-models.pdf]
