# Supplementary material for: Effective Representations of Clinical Notes
Source: arXiv:1705.07025 source file (2018-08-16)
Supplement: Supplementary file 3 [file appendix_old.tex]

\section{Details on note-level evaluation}\label{sec:app-i2b2}
The publicly available dataset contains approximately 1,230 clinical notes (730 for training and 500 for testing) and 15 targets. The targets are phenotypes such as \textit{Asthma, Obesity}, etc, and they all have 4 possible classes: Present, Absent, Questionable and Unmentioned. 
% The dataset is divided in two sub-tasks which contain the same inputs/outputs but differ on the method used to label the data. The first one is the \textit{textual task} for which labels are attributed from explicit mention in the notes; for the \textit{intuitive task} however, classification was done by using doctors' intuition and judgment based on the clinical notes. The latter is thus supposed to be more complex and require a higher level semantic understanding of the input.


The notes were processed with the Shah Lab annotator so that it had the exact same format as the notes in the STRIDE database. From the original training set, we randomly subsampled a validation set containing 20\% of the data. We report only the classification models that yielded the highest accuracies: a Random Forest with 10 trees was used for the baseline representation (bag-of-words) and a $k$-Nearest Neighbors for all other inputs ($k$ was chosen by cross-validation on the remaining training data).


\begin{table}[h]
\centering

\begin{tabular}{|l|c|c|c|}
\hline
\textbf{Embedding method}                     & \textbf{Aggregation} & \textbf{Textual}   & \textbf{Intuitive}  \\ \hline
Baseline                       & all           & \textbf{0,807} & \textbf{0,803}  \\ \hline
GloVe-300-W7-R2                    & max         & 0,784          & \textbf{0,785}  \\ \hline
GloVe-300-W7-R2                 & min         & 0,772          & 0,774           \\ \hline
GloVe-300-W7-R2                   & mean        & 0,754          & 0,759           \\ \hline
GloVe-300-W7-R2                   & sum         & 0,763          & 0,765           \\ \hline
GloVe-500-W7-R2                    & max         & \textbf{0,788} & 0,776           \\ \hline
GloVe-300-W10-R2                   & max         & 0,749          & 0,758           \\ \hline
GloVe-300-W10-R1                         & max         & 0,77           & 0,764           \\ \hline
GloVe-300-W4-R3                         & max         & 0,769          & 0,783           \\ \hline
MCEMJ                         & max         & 0,775          & 0,761           \\ \hline
Cross-channel            & max         & 0,775          & 0,759           \\ \hline
MaxGRU300                & max         & 0,780          & 0,783           \\ \hline
MaxGRU200-MCEMJ & max         & 0,773          & 0,769           \\ \hline
\end{tabular}
\caption{Micro-averaged F1 scores on the \textit{validation} set for several word embeddings}
\label{table:i2b2-details}
\end{table}

\section{Patient-level evaluation with 2,000 patients}
\label{app:2000}

We report, for reference, the results of some of our models when the evaluation task is trained on 2,000 patients instead of 500. As stated earlier, the baseline could not converge in this setting. What's reported is still the average AUROC across 20 training groups, as well as the standard error.

\begin{table}[H]
\centering
\begin{tabular}{|l|c|c|c|}
\hline
\textbf{Method}                   & \multicolumn{1}{l|}{\textbf{Death}} & \multicolumn{1}{l|}{\textbf{Admission}} & \multicolumn{1}{l|}{\textbf{ER Visit}} \\ \hline
\textbf{Baseline}                 & NA                                  & NA                                      & NA                                     \\ \hline
\textbf{GloVe-300-W7-R2  + MCEMJ} & 0.864 (0.001)                       & 0.783 (0.002)                           & \textbf{0.78 (0.001)}                  \\ \hline
\textbf{MaxGRU300}                & \textbf{0.866 (0.001)}              & \textbf{0.791 (0.001)}                  & 0.768 (0.002)                          \\ \hline
\textbf{MaxGRU600}                & 0.864 (0.001)                       & 0.789 (0.001)                           & 0.775 (0.001)                          \\ \hline
\textbf{MaxGRU500-MCEMJ}          & 0.849 (0.001)                       & 0.775 (0.002)                           & 0.766 (0.001)                          \\ \hline
\textbf{MaxGRU200-MCEMJ}          & 0.854 (0.001)                       & 0.782 (0.002)                           & 0.767 (0.001)                          \\ \hline
\end{tabular}
\caption{Evaluation on prediction of mortality and hospital utilization.}
\end{table}

\begin{table}[H]
\centering
\begin{tabular}{|l|c|c|c|c|c|c|}
\hline
\textbf{Method}                   & \textbf{Thyroid}       & \textbf{Dysrhythmias}  & \textbf{Diabetes}      & \textbf{Spondylosis}   & \textbf{LMD}           & \textbf{Hypertension}  \\ \hline
\textbf{Baseline}                 & NA                     & NA                     & NA                     & NA                     & NA                     & NA                     \\ \hline
\textbf{GloVe  + MCEMJ} & 0.704 (0.003)          & 0.728 (0.002)          & 0.735 (0.002)          & 0.73 (0.001)           & 0.706 (0.002)          & 0.719 (0.002)          \\ \hline
\textbf{MaxGRU300}                & 0.744 (0.002)          & 0.738 (0.013)          & 0.77 (0.002)           & 0.761 (0.001)          & 0.749 (0.001)          & 0.768 (0.001)          \\ \hline
\textbf{MaxGRU600}                & \textbf{0.759 (0.002)} & 0.738 (0.013)          & \textbf{0.785 (0.002)} & \textbf{0.766 (0.001)} & \textbf{0.752 (0.001)} & \textbf{0.778 (0.002)} \\ \hline
\textbf{MaxGRU500-MCEMJ}          & 0.685 (0.003)          & 0.737 (0.003)          & 0.757 (0.001)          & 0.745 (0.001)          & 0.737 (0.001)          & 0.768 (0.001)          \\ \hline
\textbf{MaxGRU200-MCEMJ}          & 0.706 (0.002)          & \textbf{0.741 (0.001)} & 0.761 (0.001)          & 0.755 (0.001)          & 0.743 (0.002)          & 0.768 (0.001)          \\ \hline
\end{tabular}
\caption{Evaluation on prediction of future diseases.}
\end{table}
